# Supplementary material for: Nonlinear dynamics and magneto-elasticity of nanodrums near the phase transition
Source: arXiv:2309.09672 source file (2023-09-18)
Supplement: Supplementary file 1 [file SI_Nonlin_FePS3__2_.pdf]

# SUPPLEMENTARY INFORMATION: Nonlinear dynamics and magneto-elasticity of nanodrums near the phase transition

Makars Šiškins,[1,2,*] Ata Keşkekler,[1] Maurits Houmes,[3] Samuel Mañas-Valero,[3,4] Eugenio Coronado,[4] Yaroslav M. Blanter,[3] Herre S. J. van der Zant,[3] Peter G. Steeneken,[1,3] and Farbod Alijani[1,*]

[1] *Department of Precision and Microsystems Engineering, Delft University of Technology, Mekelweg 2, 2628 CD, Delft, The Netherlands*
[2] *Institute for Functional Intelligent Materials, National University of Singapore, 4 Science Drive 2, Singapore 117544, Singapore*
[3] *Kavli Institute of Nanoscience, Delft University of Technology, Lorentzweg 1, 2628 CJ, Delft, The Netherlands*
[4] *Instituto de Ciencia Molecular (ICMol), Universitat de València, c/Catedrático José Beltrán 2, 46980 Paterna, Spain*

## CONTENTS

Supplementary Note 1. Mechanical dissipation in linear and nonlinear regime 2

Supplementary Note 2. Renormalization of the Duffing response through phase transition 2

Supplementary Note 3. Reproducibility of the results 2

Supplementary Note 4. Extracting experimental parameters 5

Supplementary Note 5. Magnetostrictive model: derivation of nonlinear stiffness and damping 6
Dynamics of antiferromagnetic order parameter 6
Steady-state equations 7

Supplementary References 11

* e-mail: makars@nus.edu.sg; f.alijani@tudelft.nl

## Supplementary Note 1. MECHANICAL DISSIPATION IN LINEAR AND NONLINEAR REGIME

We plot the mechanical dissipation, the inverse of a quality factor $Q^{-1}(T)$ of the MLG/FePS$_3$ resonator from Fig. 1 of the main text in Supplementary Fig. 1a. A notable peak is visible at $T_{\mathrm{N}} = 110$ K. We attribute this observation to an increase of the thermoelastic damping [1, 2] expected near the $T_{\mathrm{N}}$ in magnetic resonators as $Q^{-1} \propto c_v(T)T$, where $c_v(T)$ is the temperature-dependent specific heat of FePS$_3$ [3–5].

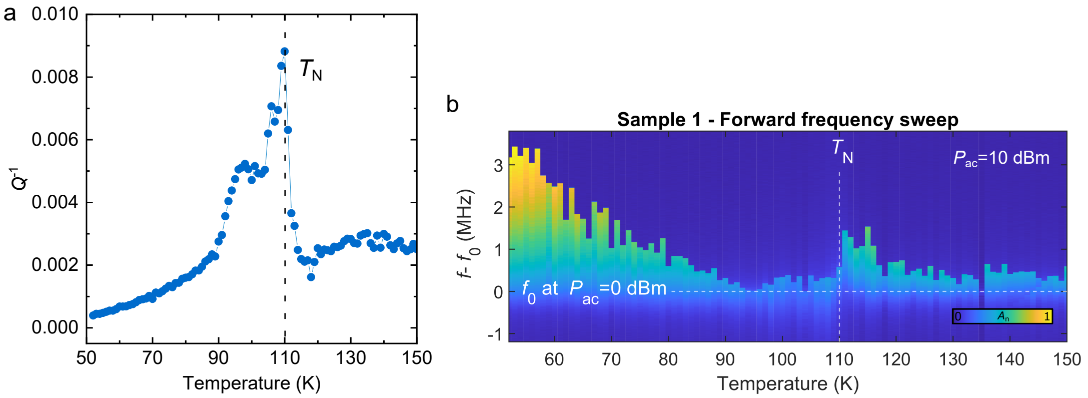


SUPPLEMENTARY FIG. 1. Measured mechanical dissipation in linear and nonlinear regime. **a** Inverse quality factor $Q^{-1}$ of the MLG/FePS$_3$ membrane (sample 1) from Fig. 1 of the main text. **b** Normalized amplitude at 10 dBm drive for the forward frequency sweep measurement of the same sample from Fig. 1 of the main text.

The mechanical dissipation of the same resonator from Fig. 1 of the main text at higher drive level and in nonlinear regime ($P_{\mathrm{ac}} = 10$ dBm) is also manifested as a decrease of maximal measured amplitude for forward frequency sweep, which we plot in Supplementary Fig. 1b. A notable anomaly is visible at $T_{\mathrm{N}} = 110$ K, which we attribute to the observation of increased nonlinear damping as further discussed in the main text.

## Supplementary Note 2. RENORMALIZATION OF THE DUFFING RESPONSE THROUGH PHASE TRANSITION

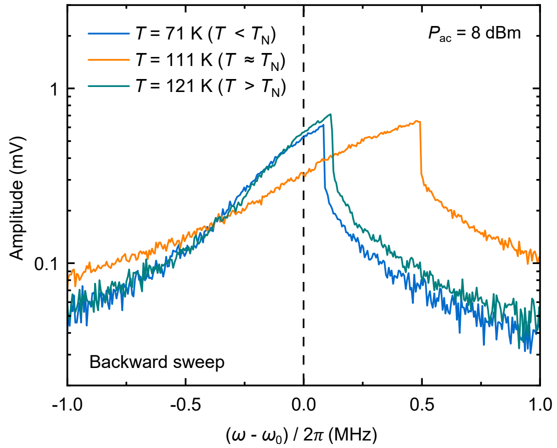


SUPPLEMENTARY FIG. 2. The measured resonance peak amplitudes at 8 dBm drive for 71, 111 and 121 K temperature points from Fig. 2c of the main text, superimposed for comparative purposes.

## Supplementary Note 3. REPRODUCIBILITY OF THE RESULTS

We have performed additional control experiments on multiple FePS$_3$/MLG samples, summarised in Supplementary Fig. 3, using both optothermal and electrostatic excitation, where an AC voltage $V_{\mathrm{ac}}$ signal is applied between the Si

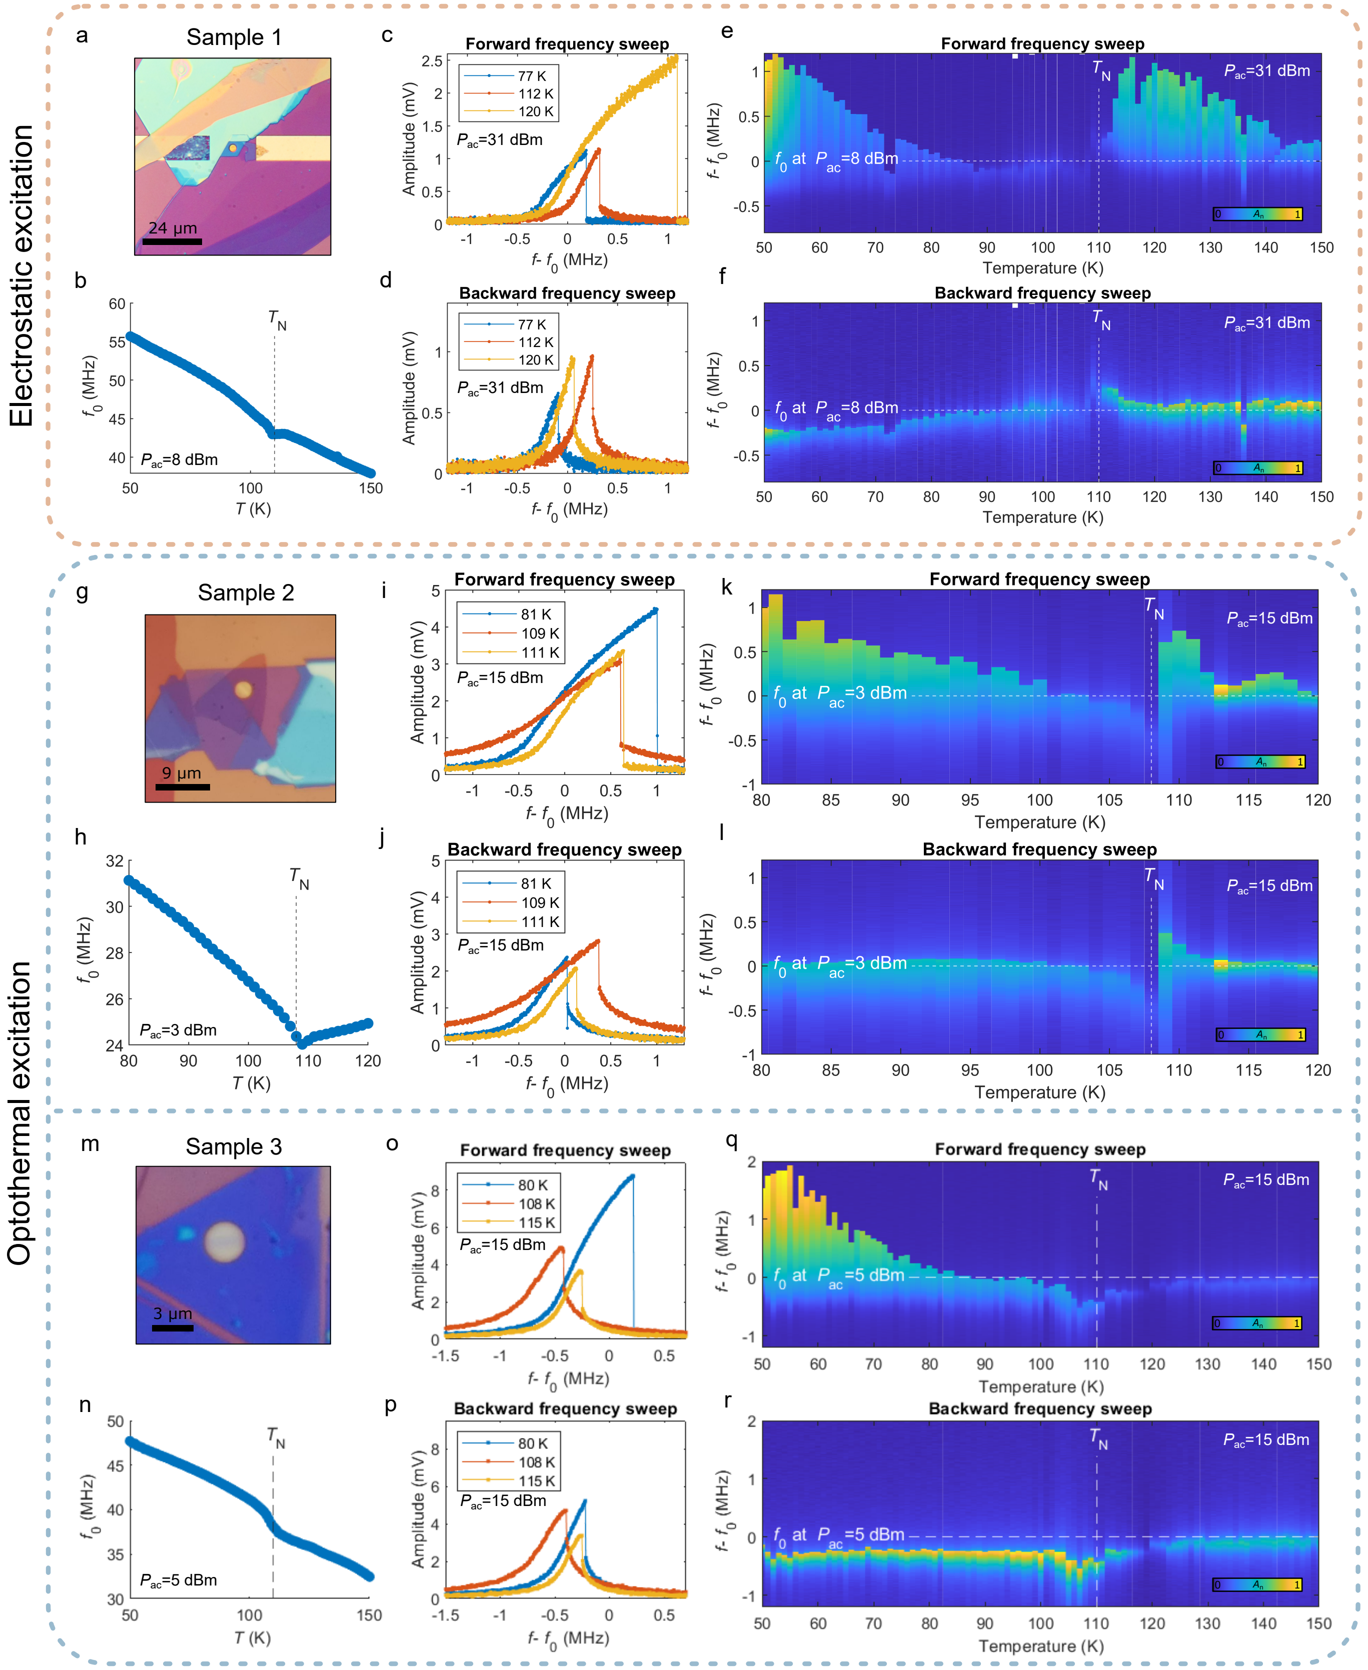


SUPPLEMENTARY FIG. 3. Additional measurements on $FePS_3$/MLG samples. **a-f** The $FePS_3$/MLG sample from the main text measured under electrostatic excitation $V_{ac}$ applied to the bottom gate electrode with a DC offset $V_{dc} = 10$ V. **a** Optical image of the sample. **b** Measured resonance frequency of the fundamental membrane mode $f_0$ as a function of temperature. **c-f** The Duffing effect and amplitude-frequency branches of the resonance peak at higher drive ($P_{ac}$) measured for forward (**c**) and backward frequency sweep. **e-f** The colour map of the normalized amplitude measured as a function of temperature in forward (**e**) and backward (**f**) frequency sweep regime around linear resonance frequency $f_0$ from (b). **g-l** and **m-r** are two additional $FePS_3$/MLG samples measured under opto-thermal excitation. **g-l** and **m-r** follow the same structure as (a-f).

backgate of the chip and the conducting top layer of MLG. Since we obtain similar results for the electrostatic drive as for optothermal drive we conclude that the reported observations are intrinsic to the resonator and not related to the driving mechanism.

We note that the qualitatively different behaviour of $f_0(T)$ in Supplementary Fig. 3 can be well understood considering the interplay between thermal expansion coefficients of materials involved: $FePS_3$, graphene and Si substrate. The resonance frequency of a heterostructure membrane $f_{0,\mathrm{h}}(T)$ can be modelled considering the total thermally accumulated tension of the $FePS_3$/MLG heterostructure as a sum of individual tensions in each layer, assuming that the slippage between the layers is negligible [4]:

$$
\begin{aligned}
f_{0,\mathrm{h}}(T) &= \sqrt{\left(\frac{2.4048}{2\pi r}\right)^2 \frac{n_{\mathrm{th}}(T)}{\rho h} + f_0^2(T_0)} \\
&= \sqrt{\left(\frac{2.4048}{2\pi r}\right)^2 \frac{1}{\rho_1 h_1 + \rho_2 h_2}\left[\frac{E_1 h_1}{(1-\nu_1)}\epsilon_{\mathrm{th},1}(T) + \frac{E_2 h_2}{(1-\nu_2)}\epsilon_{\mathrm{th},2}(T)\right] + f_0^2(T_0)}.
\end{aligned}
\tag{1}
$$

where $f_0(T_0)$ is the resonance frequency at a reference temperature $T_0$ (e.g. room temperature) due to the contribution of the pre-tension and the bending rigidity, $E$ the Young's modulus, $\nu$ the Poisson ratio, $h$ the layer thickness, $\rho$ the mass density, $n_{\mathrm{th}}(T) = \frac{Eh}{(1-\nu)}\epsilon_{\mathrm{th}}$ the thermally accumulated tension, $\epsilon_{\mathrm{th}} = -\int_{T_0}^{T_i} (\alpha_{\mathrm{material}}(T) - \alpha_{\mathrm{Si}}(T))\,\mathrm{d}T$ the thermal strain at an arbitrary temperature $T_i$ [3, 6], $\alpha_{\mathrm{Si}}(T)$ the literature values for thermal expansion coefficient of Si substrate [7], and $\alpha_{\mathrm{material}}(T)$ the temperature dependent thermal expansion coefficient of either $FePS_3$ [3] or graphene [8], shown in Supplementary Fig. 4a.

Thus, we attribute the observed differences in $f_0(T)$ trends to a large contribution of $\alpha_{\mathrm{MLG}}(T)$ to the total in-plane stress of the membrane, especially at $T < T_{\mathrm{N}}$, prominence of which depends on the material's thickness ratio. We demonstrate this by plotting the model of equation (1) in Fig. 4b for two different thicknesses of MLG layer. We use $E_{\mathrm{FePS_3}} = 103$ GPa, $\rho_{\mathrm{FePS_3}} = 3375$ kgm$^{-3}$, $\nu_{\mathrm{FePS_3}} = 0.304$ for $FePS_3$ [3]; and $E_{\mathrm{MLG}} = 1$ TPa, $\rho_{\mathrm{MLG}} = 2260$ kgm$^{-3}$, $\nu_{\mathrm{MLG}} = 0.19$ for graphene [9]; From Fig. 4b it is apparent that for the thinner MLG layer in the heterostructure, $f_0(T)$ is expected to monotonically increase with decreasing temperature, similar to samples 1, 3 from Supplementary Fig. 3, while for the thicker MLG layer case, non-monotonic behaviour can be expected, similar to samples 2 from the same figure.

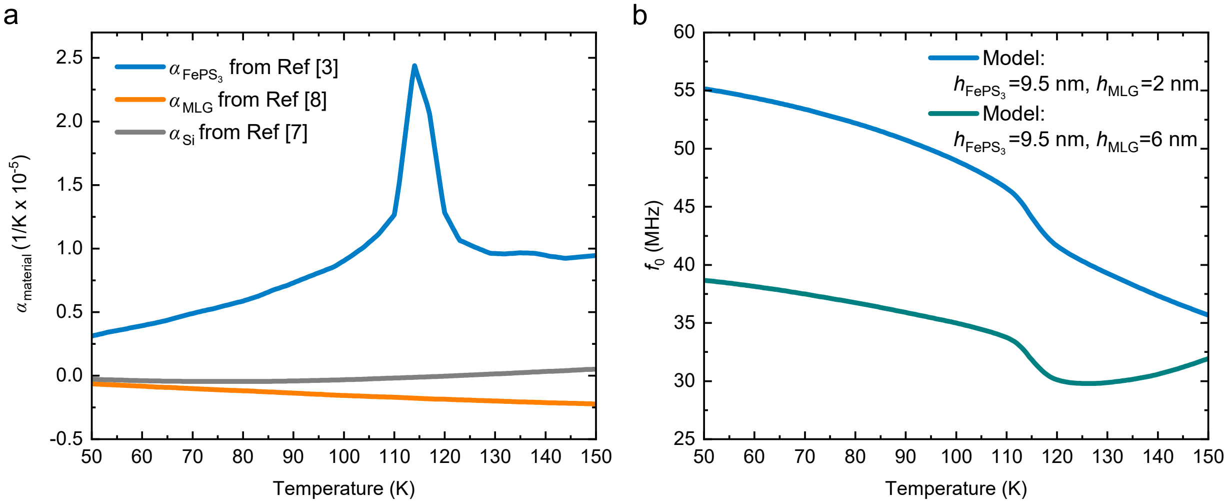


SUPPLEMENTARY FIG. 4. Temperature dependence of thermal expansion and resonance frequency of $FePS_3$/MLG heterostructure membranes. **a** Linear thermal expansion coefficients of $FePS_3$ [3], graphene [8] and Si substrate [7]. **b** The resonance frequency model of equation (1) as a function of temperature and thicknesses of $FePS_3$ and MLG, calculated using the data from (a).

## Supplementary Note 4. EXTRACTING EXPERIMENTAL PARAMETERS

In the main text, to monitor the change in the stiffness and dissipation of the resonator, we fit the experimental frequency responses to the equation (12), to extract $Q$, $\gamma$, $\xi_{\mathrm{nl}}$, $F_\omega/m$ and $\omega_0$. The fitting is done sequentially. First, $Q$ factors are extracted from the linewidths of linear resonance curves at low drive levels, before the onset of nonlinearity. Next, $\omega_0$ is extracted from the peak frequency at low drive levels, assuming it stays constant with increasing drive levels. However, we have sometimes also observed dependency of the fundamental frequency on drive level, possibly due to overheating from the optothermal drive. Thus, we extracted $\omega_0$ for each drive level separately. At the drive levels where the response is nonlinear, we correct for the $\omega_0$ using the inflection of the nonlinear resonance curve, such that $f_{\mathrm{dd}}(\omega) = \frac{d^2 a_{\mathrm{s}}}{d\omega^2}$ where $f_{\mathrm{dd}}(\omega_0) \approx 0$ or the saddle-node bifurcation of the lower solution branch obtained in the reverse sweep.

After obtaining $Q$ and $\omega_0$, it is possible to extract $F_\omega/m$ by fitting the off-resonance response to a harmonic oscillator model, such that $\ddot{x} + \frac{\omega_0}{Q}\dot{x} + \omega_0^2 x = \frac{F_\omega}{m}$. After obtaining all the linear parameters, we extract nonlinear parameters $\gamma$ and $\xi_{\mathrm{nl}}$. Normalized Duffing coefficient $\gamma$ is estimated by using the slope of the square of the frequency response since $\gamma = (8\omega_0/3)(\omega_{\mathrm{max}} - \omega_0)/a^2_{\mathrm{s,max}}$ [10], where $\omega_{\mathrm{max}}$ is the frequency and $a_{\mathrm{max}}$ is the amplitude of the experimental nonlinear resonance peak. Finally, we find $\xi_{\mathrm{nl}}$ by matching the peak amplitude i.e. saddle-node bifurcation of the higher solution branch, and by using an optimizer that minimizes the objective $f_{\mathrm{obj}} = |a^{\mathrm{sim}}_{\mathrm{s,max}}(\xi_{\mathrm{nl}}) - a_{\mathrm{s,max}}|$, where $a^{\mathrm{sim}}_{\mathrm{s,max}}$ is the peak amplitude of the simulated model. In Supplementary Fig. 5, we provide additional examples of the fitted curves for convenience.

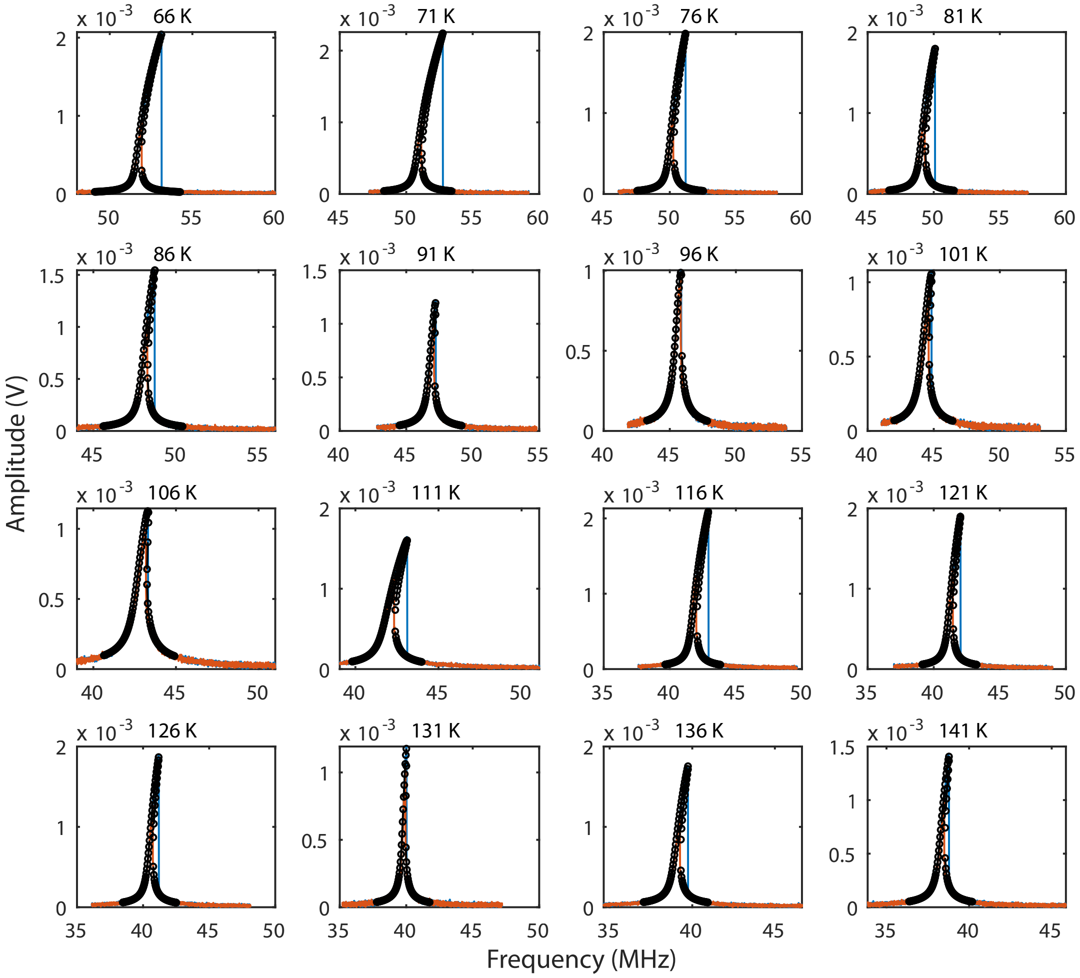


SUPPLEMENTARY FIG. 5. Model fits to the experimental data for various temperatures at 10 dBm drive level. The blue line is the experimental forward frequency sweep response, whereas the orange line is in the reverse sweep response. Black circles are the simulated model response with fitted parameters.

## Supplementary Note 5. MAGNETOSTRICTIVE MODEL: DERIVATION OF NONLINEAR STIFFNESS AND DAMPING

### Dynamics of antiferromagnetic order parameter

In the derivation of antiferromagnetic order parameter relaxation dynamics, we follow closely the approach of Landau-Khalatnikov [11] and Belov-Kataev-Levitin [12, 13]. Total potential energy of the system can be written down as follows:

$$U_{\mathrm{T}} = U_{\mathrm{el}} + U_{\mathrm{m}} + U_{\mathrm{ms}}, \tag{2}$$

where $U_{\mathrm{el}}$ is elastic potential energy, $U_{\mathrm{m}}$ free energy of an antiferromagnet and $U_{\mathrm{ms}}$ is magnetostrictive coupling energy term. These take form of:

$$\begin{aligned} U_{\mathrm{el}} &= \frac{k_1}{2}x^2 + \frac{k_3}{4}x^4 \\ U_{\mathrm{m}} &= U_{\mathrm{m},0} + \frac{A}{2}L^2 + \frac{B}{4}L^4 \\ U_{\mathrm{ms}} &= \frac{\lambda_{ij}}{2}\sigma_{ij}(x)L^2, \end{aligned} \tag{3}$$

where $k_1$ and $k_3$ are linear and nonlinear stiffness, $U_{\mathrm{m},0}$ is the magnetic free energy in a paramagnetic state, $L = M_1 - M_2$ is an antiferromagnetic order parameter along the easy-axis of antiferromagnet defined as a difference of counter-aligned spin sub-lattice magnetisations $M_{1,2}$, while $A$ and $B$ are phenomenological constants, $\lambda_{ij}$ tensor of phenomenological magnetostrictive coefficient, $\sigma_{ij}(x)$ is stress tensor modulated by the membrane deflection $x$. For notational convenience, we write $\lambda_{ij}$ in dropping the third and fourth index of $\lambda_{ijkl}$ as only the component where $kl$ corresponds to the easy axis contribution.

Let us first consider magnetic energy terms $U_{\mathrm{m}} + U_{\mathrm{ms}}$ that describe the antiferromagnetic phase for uni-axial magnetic anisotropy:

$$U_{\mathrm{m}} + U_{\mathrm{ms}} = U_{\mathrm{m},0} + \frac{A}{2}L^2 + \frac{B}{4}L^4 + \frac{\lambda}{2}L^2\sigma(x), \tag{4}$$

where $B > 0$, $\sigma(x) = \sigma_{xx} = \sigma_{yy}$ is in-plane bi-axial stress and $\lambda$ the specific magnetostriction coefficient of $\lambda_{ij}$ tensor that describes the coupling of in-plane membrane stress to order parameter in the direction of the easy axis $L$. In zero stress conditions $\sigma = 0$ the energy minimum thus shall have extrema that satisfy $\frac{\partial(U_{\mathrm{m}} - U_{\mathrm{m},0})}{\partial L} = 0$, where $A > 0$ condition describes a disordered (paramagnetic) phase and $A < 0$ condition - an ordered (antiferromagnetic) phase. Consequently, $A = 0$ describes the transition between these phases. We thus define antiferromagnetic transition temperature or Néel temperature $T_{\mathrm{N}}$ such that it leads to $A = 0$ at $T_{\mathrm{N}}$ as:

$$A = a(T - T_{\mathrm{N}})^{2\beta}, \tag{5}$$

where $a$ is a positive phenomenological constant, $T$ is temperature and $\beta = 0.5$ the critical exponent [14]. By plugging equation (5) to (3), we write a full equation for total potential energy:

$$\begin{aligned} U_{\mathrm{T}} &= U_{\mathrm{el}} + U_{\mathrm{m}} + U_{\mathrm{ms}} \\ &= \left[\frac{k_1}{2}x^2 + \frac{k_3}{4}x^4\right] + \left[U_{\mathrm{m},0} + \frac{a}{2}\left(T - T_{\mathrm{N}}\right)L^2 + \frac{B}{4}L^4\right] + \left[\frac{\lambda}{2}L^2\sigma(x)\right], \end{aligned} \tag{6}$$

We minimize $U_{\mathrm{T}}$ with respect to $L$ to find the values of the order parameter at the ground state under the static stress condition $\sigma = \sigma_0$. This leads to:

$$\frac{\partial U_{\mathrm{T}}}{\partial L} = a\left(T - T_{\mathrm{N}}\right)L + BL^3 + \lambda L\sigma_0 = 0, \tag{7}$$

where $\sigma_0$ is the static stress term of the total in-plane membrane stress, defined as, assuming flat membrane case and $x \approx a_{\mathrm{s}}\cos(\omega t)$ [15, 16]:

$$\begin{aligned} \sigma(x) &= \sigma_{\mathrm{p}} + \frac{Ec_3}{2r^2}x^2 \\ &= \left[\sigma_{\mathrm{p}} + \frac{Ec_3}{4r^2}a_{\mathrm{s}}^2\right] + \left[\frac{Ec_3}{4r^2}a_{\mathrm{s}}^2\cos(2\omega t)\right] \\ &= \sigma_0 + \sigma_\omega(t), \end{aligned} \tag{8}$$

where $\sigma_{\mathrm{p}}$ is the pre-stress in the membrane due to the fabrication process, $\sigma_\omega(t)$ the dynamic stress terms, $E$ the Young's modulus, $r$ the membrane radius, $a_{\mathrm{s}}$ the steady-state amplitude, $t$ the time, $\omega$ the drive frequency, and $c_3$ the geometric numerical factor that depends on membrane's Poisson ratio [17].

Equation (7) then leads to the antiferomagnetic order parameter at the ground state:

$$L_0 = \pm\sqrt{\frac{a(T_{\mathrm{N}} - T) - \lambda\sigma_0}{B}} = \pm\sqrt{\frac{a(T_{\mathrm{N}}^* - T)}{B}}. \tag{9}$$

Consequently, one can show that magnetostriction produces the shifted Néel temperature $T_N^*$ as a function of $\sigma_0$:

$$T_{\mathrm{N}}^* = T_{\mathrm{N}} - \frac{\lambda\sigma_0}{a}. \tag{10}$$

In contrast, a stressed antiferromagnet in motion satisfies the following relation between $L$ and $T_{\mathrm{N}}$:

$$L(t)^2 = \frac{a(T_{\mathrm{N}} - T) - \lambda\left(\sigma_0 + \sigma_\omega(t)\right)}{B} \cong \left(L_0 + L_\omega(t)\right)^2, \tag{11}$$

where $L_\omega(t)$ is the dynamic term of the antiferromagnetic order parameter $L$. When the membrane is in motion, the time dependence of $L$ is related to the energy $U_{\mathrm{T}}$ by the kinetic equation [11–13]:

$$\frac{dL}{dt} = -\kappa\frac{\partial U_{\mathrm{T}}}{\partial L}, \tag{12}$$

where $\kappa$ is the kinetic coefficient, that is assumed to be free of anomalies near $T_{\mathrm{N}}$ [11]. Since, from equation (11), $L(t) = L_0 + L_\omega(t)$ is a sum of the equilibrium $L_0$ and the additional dynamic term $L_\omega(t)$, produced by the small oscillating stresses $\sigma_\omega(t)$, we can expand $\frac{\partial U_{\mathrm{T}}}{\partial L}$ using Taylor series around $L_0$:

$$\frac{dL}{dt} \cong -\kappa\left[\frac{\partial U_{\mathrm{T}}}{\partial L}|_{L_0} + \frac{\partial^2 U_{\mathrm{T}}}{\partial L^2}|_{L_0}(L - L_0) + ...\right], \tag{13}$$

and obtain, assuming $L_\omega \ll L_0$:

$$-\frac{dL_\omega}{dt} \cong 2\kappa B L_0^2 L_\omega + \kappa\lambda L_0 \sigma_\omega(t). \tag{14}$$

As originally shown by Landau and Khalatnikov [11], the time constant $\tau$, that describes the relaxation of an antiferromagnetic order parameter due to its dynamic term [12, 13], can be found from equation (14) as:

$$\tau = \begin{cases} \frac{1}{2\kappa a\left(T_{\mathrm{N}}^* - T\right)} & T < T_{\mathrm{N}}^* \\ \infty & T > T_{\mathrm{N}}^*, \end{cases} \tag{15}$$

which further simplifies equation (14) to:

$$\dot{L}_\omega + \frac{L_\omega}{\tau} + \kappa\lambda L_0 \sigma_\omega(t) = 0. \tag{16}$$

**Steady-state equations**

We use the method of harmonic balancing to solve for the steady-state amplitude of equation (4) in the main text. We approximate the motion by a single harmonic such that $x \approx a_{\mathrm{s}}\cos(\omega t + \psi)$ where $a_{\mathrm{s}}$ is the steady-state amplitude. In order to obtain the steady-state response of the mechanical degree of freedom $x$, that is coupled to the magnetic order, we define the Lagrangian $\mathcal{L} = \frac{1}{2}m\dot{x}^2 - U_{\mathrm{T}}$, and use the Euler-Lagrange equation as follows:

$$\frac{d}{dt}\frac{\partial \mathcal{L}}{\partial \dot{x}} - \frac{\partial \mathcal{L}}{\partial x} = 0, \tag{17}$$

which yields:

$$m\ddot{x} + k_1 x + k_3 x^3 + \frac{\lambda}{2}(L_0 + L_\omega)^2\frac{\partial \sigma}{\partial x} = 0, \tag{18}$$

where $k_1 = m\omega_0^2$. Assuming that $L_0 \gg L_\omega$ and including linear dissipation related to the quality factor $Q$, nonlinear damping of van der Pol type [18–20] $\eta_{\rm nl}$ and periodic forcing with the amplitude $F_\omega$ with frequency $\omega$ and phase $\psi$, coupled equations of motion can be written in the following form:

$$\begin{cases} m\ddot{x} + k_1 x + k_3 x^3 + \frac{\lambda}{2}\left(L_0^2 + 2L_0 L_\omega\right)\frac{\partial \sigma}{\partial x} = F_\omega \cos\left(\omega t + \psi\right) - \frac{m\omega_0}{Q}\dot{x} - \eta_{\rm nl} x^2 \dot{x}, \\ \dot{L}_\omega + \frac{L_\omega}{\tau} + \kappa\lambda L_0 \sigma_\omega(t) = 0. \end{cases} \tag{19}$$

To solve for the steady-state response of the mechanical degree of freedom coupled to the magnetic order, we start by solving the first-order differential equation (19). Using equations (15) and (8), we obtain the steady-state solution for $L_\omega$ in terms of $\tau$:

$$\begin{aligned} L_{\omega,\rm ss} &= -\lambda\kappa L_0 \frac{Ec_3}{4r^2}\left[\cos\left(2\omega t\right) + 2\tau\omega \sin\left(2\omega t\right)\right]\frac{\tau}{1+4\tau^2\omega^2} a_{\rm s}^2 \\ &= -\lambda\kappa L_0 \left[\sigma_\omega(t) - \tau\frac{\partial \sigma_\omega(t)}{\partial t}\right]\frac{\tau}{1+4\tau^2\omega^2}. \end{aligned} \tag{20}$$

Consequently, to apply the method of harmonic balancing to the equation (19), we keep the assumption of periodic motion at the steady state in the form of $x = a_{\rm s}\cos\omega t$ and plug in the steady state solution of $L_\omega$, such that $L_\omega = L_{\omega,\rm ss}$. Considering only the fundamental harmonic $\omega$ and discarding higher order harmonics, we find:

$$\begin{aligned} &\left[\left(\frac{3k_3}{4} - \frac{\lambda^2}{4B}\frac{E^2c_3^2}{4r^4}\frac{1}{(1+4\tau^2\omega^2)}\right)a_{\rm s}^3 + m(\omega_0^2-\omega^2)a_{\rm s}\right]\cos\omega t - \\ &\left[\left(\eta_{\rm nl} + \frac{\lambda^2\omega}{2B}\frac{E^2c_3^2}{r^4}\frac{\tau}{(1+4\tau^2\omega^2)}\right)a_{\rm s}^3 + \frac{m\omega_0\omega}{Q}a_{\rm s}\right]\sin\omega t = F_\omega\cos\psi\cos\omega t - F_\omega \sin\psi\sin\omega t. \end{aligned} \tag{21}$$

We equate the coefficients of the fundamental harmonic, namely $\sin\omega t$ and $\cos\omega t$ on both sides and obtain the following steady-state amplitude equation:

$$\begin{aligned} &\left(\left(\frac{3k_3}{4} - \frac{\lambda^2}{16B}\frac{E^2c_3^2}{r^4}\frac{1}{(1+4\tau^2\omega^2)}\right)a_{\rm s}^3 + m(\omega_0^2-\omega^2)a_{\rm s}\right)^2 \\ &+\left(\left(\eta_{\rm nl} + \frac{\lambda^2\omega}{2B}\frac{E^2c_3^2}{r^4}\frac{\tau}{(1+4\tau^2\omega^2)}\right)a_{\rm s}^3 + \frac{m\omega_0}{Q}a_{\rm s}\right)^2\omega^2 = F_\omega^2, \end{aligned} \tag{22}$$

where $\omega_0^2 = \frac{1}{m}\left(k_1 + \lambda L_0^2 \frac{Ec_3}{2r^2}\right)$ the re-normalized resonance frequency. From the steady-state amplitude equation, it is possible to see that the coupling to the magnetic order leads to a re-normalized nonlinear damping term $\eta_{\rm nl}^*$ of van der Pol type [18–20] at $T < T_{\rm N}^*$ such that:

$$\boxed{\eta_{\rm nl}^* = \begin{cases} \eta_{\rm nl} + \frac{\lambda^2}{2B}\frac{E^2c_3^2}{r^4}\frac{\tau}{(1+4\tau^2\omega^2)} & T < T_{\rm N}^* \\ \eta_{\rm nl} & T > T_{\rm N}^* \end{cases}}. \tag{23}$$

Similarly, due to coupling, the nonlinear stiffness of the Duffing type $k_3^*$ is re-scaled, such that:

$$\boxed{k_3^* = \begin{cases} k_3 - \frac{\lambda^2}{12B}\frac{E^2c_3^2}{r^4}\frac{1}{(1+4\tau^2\omega^2)} & T < T_{\rm N}^* \\ k_3 & T > T_{\rm N}^* \end{cases}}, \tag{24}$$

and the linear stiffness $k_1^*$ as:

$$\boxed{k_1^* = \begin{cases} k_1 + \lambda L_0^2\frac{Ec_3}{2r^2} & T < T_{\rm N}^* \\ k_1 & T > T_{\rm N}^* \end{cases}}, \tag{25}$$

Thus, the dynamics of the membrane can be effectively described using a single nonlinear differential equation with renormalized linear stiffness as well as Duffing and van der Pol nonlinear damping terms:

$$m\ddot{x} + k_1^* x + k_3^* x^3 = F_\omega\cos\left(\omega t\right) - \frac{m\omega_0}{Q}\dot{x} - \eta_{\rm nl}^* x^2\dot{x}, \tag{26}$$

where $\omega_0^2 = \frac{k_1^*}{m}$ is the renormalized resonance frequency.

It is worth noting from equation (23) that $\eta_{\rm nl}^*$ is significant near $2\tau\omega \approx 1$ and peaks at $2\tau\omega = 1$ [21]. In previous work of Zhou et al [22], it was shown that in $FePS_3$ the longest magnetostriction-caused lattice relaxation time constant is related to modulation of monoclinic lattice angle by interlayer spin-shear coupling, which can be in the order of several tens of nanoseconds near $T_{\rm N}$ [22, 23]. These relaxation timescales are indeed expected to lead to $2\tau\omega \approx 1$ and thus hypothetically can cause significant nonlinear damping within the measured range of $\omega$.

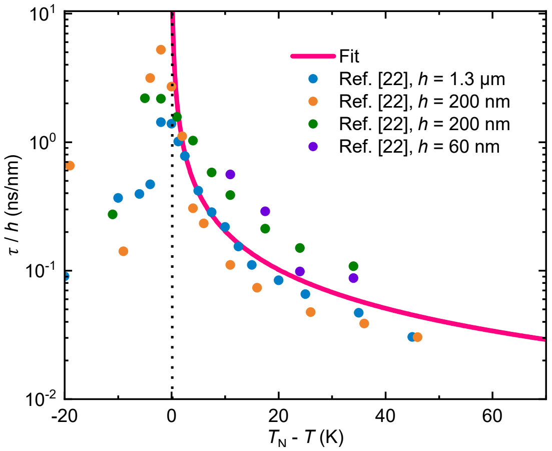


SUPPLEMENTARY FIG. 6. Thickness-normalized relaxation time constants $\tau(T)$ reported on samples of various sample thicknesses $h$ from Zhou, F. et al [22]. Solid magenta line - fit to a model of equation (15), where $T_N^* = 115$ K and $\kappa a h = 0.232 \pm 0.019$ ms$^{-1}$K$^{-1}$.

We further hypothesise that the spin-shear relaxation $\tau(T)$ from the work of Zhou et al [22] has the dominant contribution to our experimentally observed delay. By fitting experimental data from Zhou et al [22] to equation (15) (see Supplementary Fig. 6), we plot the expected temperature dependence of $k_3^*(T)$ and $\eta_{\rm nl}^*(T)$ (assuming a minor temperature dependence of $k_3(T)$ due to other effects of non-magnetic nature) in Supplementary Fig. 7 for $h = 9.5$ nm.

It is worth noting that when $\tau$ is insignificant, i.e. $\tau \approx 0$, equation (24) simplifies to:

$$\begin{cases} k_3^* = k_3 - \frac{\lambda^2}{12B}\frac{E^2 c_3^2}{r^4} & T < T_{\rm N}^* \\ k_3^* = k_3 & T > T_{\rm N}^* \end{cases}. \tag{27}$$

This will produce the corresponding behaviour near the phase transition, that we show in Supplementary Fig. 8 for $k_1^*(T)$ and $k_3^*(T)$, while the magnetic contribution to $\eta_{\rm nl}^*(T)$ becomes zero.

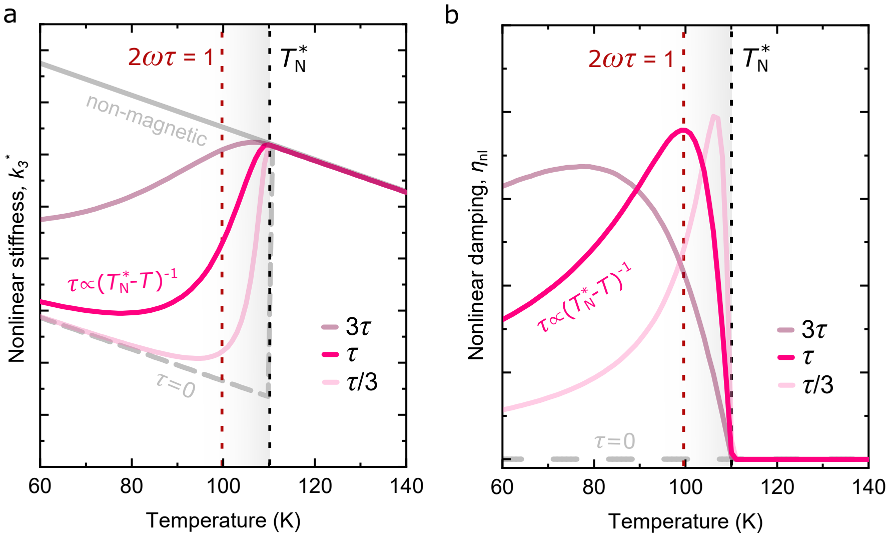


SUPPLEMENTARY FIG. 7. Re-normalized nonlinear stiffness $k_3^*$ and nonlinear damping $\eta_{\rm nl}$ calculated using equations (23) and (24) for different values of $\tau(T)$ and $2\omega_0\tau = 1$, as well as results of the fit from Supplementary Fig. 6 and $\omega(T) = \omega_0(T) = 2\pi f_0(T)$ from Fig. 1c of the main text.

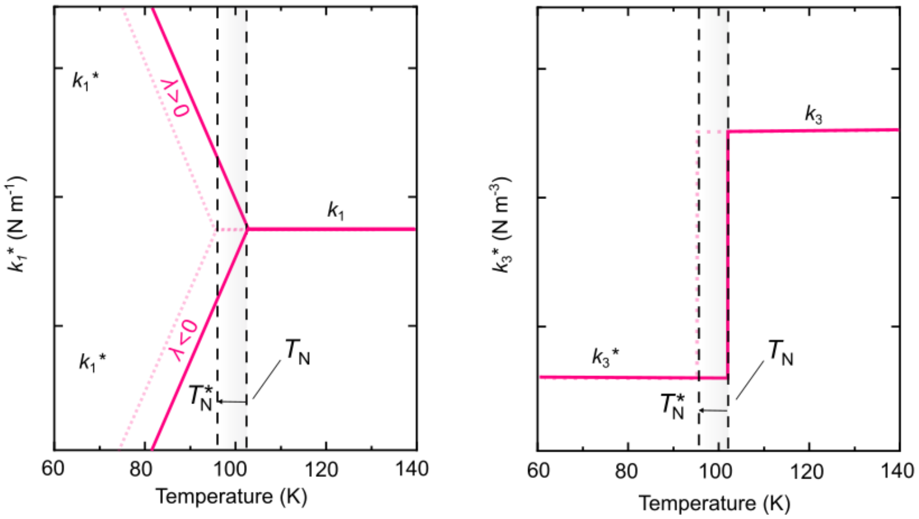


SUPPLEMENTARY FIG. 8. Re-normalized $k_1^*$ and $k_3^*$ as a function of temperature at insignificantly small $\tau$ ($\tau \approx 0$).

[1] Lifshitz, R. & Roukes, M. L. Thermoelastic damping in micro- and nanomechanical systems. *Phys. Rev. B* **61**, 5600–5609 (2000).

[2] Sun, Y. & Saka, M. Thermoelastic damping in micro-scale circular plate resonators. *J. Sound Vib.* **329**, 328–337 (2010).

[3] Šiškins, M. *et al.* Magnetic and electronic phase transitions probed by nanomechanical resonators. *Nat. Commun.* **11**, 2698 (2020).

[4] Šiškins, M. *et al.* Nanomechanical probing and strain tuning of the Curie temperature in suspended $Cr_2Ge_2Te_6$-based heterostructures. *npj 2D Mater. Appl.* **6**, 41 (2022).

[5] Šiškins, M. *et al.* Tunable strong coupling of mechanical resonance between spatially separated $FePS_3$ nanodrums. *Nano Lett.* **22**, 36–42 (2021).

[6] Morell, N. *et al.* High quality factor mechanical resonators based on $WSe_2$ monolayers. *Nano Lett.* **16**, 5102–5108 (2016).

[7] Lyon, K. G., Salinger, G. L., Swenson, C. A. & White, G. K. Linear thermal expansion measurements on silicon from 6 to 340 K. *J. Appl. Phys.* **48**, 865–868 (1977).

[8] Mann, S., Kumar, R. & Jindal, V. K. Negative thermal expansion of pure and doped graphene. *RSC Adv.* **7**, 22378 (2017).

[9] Politano, A. & Chiarello, G. Probing the Young's modulus and Poisson's ratio in graphene/metal interfaces and graphite: a comparative study. *Nano Res.* **8**, 1847–1856 (2015).

[10] Lifshitz, R. & Cross, M. C. *Nonlinear Dynamics of Nanomechanical and Micromechanical Resonators*, chap. 1, 1–52 (John Wiley & Sons, Ltd, 2008).

[11] Landau, L. D. & Khalatnikov, I. M. On the anomalous absorption of sound near a second order phase transition point. *Dokl. Akad. Nauk SSSR* **96**, 469 (1954).

[12] Belov, K. P., Kataev, G. I. & Levitin, R. Z. Anomalies in internal friction and modulus of elasticity in ferromagnetic near the Curie point. *J. Exptl. Theoret. Phys. (U.S.S.R.)* **37**, 938–943 (1959).

[13] Belov, K. P., Katayev, G. I. & Levitin, R. Z. Internal friction anomalies in ferromagnets and antiferromagnets near the Curie point. *J. Appl. Phys.* **31**, S153–S156 (1960).

[14] Landau, L. D., Pitaevskii, L. P. & Lifshitz, E. M. *Electrodynamics of continuous media*, vol. 8 (Butterworth, New York, 1984), 2 edn.

[15] Davidovikj, D. *et al.* Nonlinear dynamic characterization of two-dimensional materials. *Nat. Commun.* **8**, 1253 (2017).

[16] Zhang, X. *et al.* Dynamically-enhanced strain in atomically thin resonators. *Nat. Commun.* **11**, 5526 (2020).

[17] Davidovikj, D., Scheepers, P. H., van der Zant, H. S. J. & Steeneken, P. G. Static capacitive pressure sensing using a single graphene drum. *ACS Appl. Mater. Interfaces* **9**, 43205–43210 (2017).

[18] Keşkekler, A. *et al.* Tuning nonlinear damping in graphene nanoresonators by parametric–direct internal resonance. *Nat. Commun.* **12**, 1099 (2021).

[19] Atalaya, J., Kenny, T. W., Roukes, M. L. & Dykman, M. I. Nonlinear damping and dephasing in nanomechanical systems. *Phys. Rev. B* **94**, 195440 (2016).

[20] Catalini, L., Rossi, M., Langman, E. C. & Schliesser, A. Modeling and observation of nonlinear damping in dissipation-diluted nanomechanical resonators. *Phys. Rev. Lett.* **126** (2021).

[21] Dykman, M. I. & Krivoglaz, M. A. Spectral distribution of nonlinear oscillators with nonlinear friction due to a medium. *Phys. Status Solidi B* **68**, 111–123 (1975).

[22] Zhou, F. *et al.* Dynamical criticality of spin-shear coupling in van der Waals antiferromagnets. *Nat. Commun.* **13**, 6598 (2022).

[23] Zong, A. *et al.* Spin-mediated shear oscillators in a van der Waals antiferromagnet. *Nature* **620**, 988–993 (2023).
